# Supplementary material for: Spectral Maps for Learning on Subgraphs
Source: arXiv:2205.14938 source file (2023-01-31)
Supplement: Supplementary file 1 [file supmat.tex]

\section{Supplementary}

\textbf{Figure}: functional map between full cat and partial (cut and holes), both with mesh laplacian (Neumann) and normalized graph laplacian. Mask computed from eigenvalues \\
\textbf{Message}: On cut, the C are very similar. Surprisingly with the normalized graph laplacian the C is even sharper. This translates to better performance on the point-to-point correspondence retrieval from the C, see results section on cat 0.4 patch\_mesh 
The mask becomes more different on hole partiality. In the supplementary, I could add a table with the accuracy and other numeric evaluations of Fm with the different laplacian.

\textbf{Figure}:
{(sketch) C maps computed with different laplacian. On the left there are the maps computed with mesh laplacian (Neumann condition) and normalized graph laplacian, respectively. They are both computed on a partial mesh obtained cutting half cat. On the right a partiality given by holes}
 
 \textit{(Supplementary?)} \textbf{Figure}: full spectrum and eigenvector on karate\\ 
\textbf{Message}: Show eigenvalues with high multiplicity due to inner simmetries  

\textbf{Choice of the Laplacian} Compare different Laplacians and the structures that emerge from the functional map matrix, to motivate our choice. Note that the normalized graph Laplacian assumes that we do not have graphs with isolated nodes.

\textbf{PFM} Rodol\`{a} and colleagues~\cite{rodola2017partial} extended the functional maps framework to the case where $\N$ is a partial shape and rewrite the minimization from equation ~\ref{eq:fmap} as follows: 
\begin{align}
\label{eq:partialfmap}
     C = \underset{C \in \mathbb{R}^{k \times k}}{\arg\min} \| CF - B(\eta(\nu)) \|_{2,1} + \rho_{part}(\nu) + \rho_{corr}(C) .
\end{align}
Here we briefly describe the modifications that are relevant to our method and refer to ~\cite{rodola2017partial} for all the details.
The minimization is not only on $C$ but also on $\nu$, an indicator function representing the surface patch on $\M$ that corresponds to $\N$. We do not consider this because we work with graphs and without surfaces. The same holds for $\rho_{part}(\nu) $.
The norm adopted for the term on the probe functions is the $L_{2,1}$ matrix norm, which promotes column-sparse matrices to improve robustness to possible outliers.
$\rho_{corr}(C)$ fosters additional structure to $C$ and is defined as: 
\begin{align}
\label{eq:regularizerC}
\rho_{corr}(C) = \mu_1 \| C \odot W \|_{2}^{2} + \mu_2 \sum_{\ell \neq h} (C^{\top}C)_{\ell,j}^2 + \mu_3 \sum_{\ell} ((C^{\top}C)_{\ell,\ell} - d_{\ell})^2n ,
\end{align}
where each term has its weight $\mu_1$, $\mu_2$ and $\mu_3$.
$W$ is a mask matrix that acts through element-wise multiplication $\circ$ and encodes the relation between the eigenvalues of the two shapes, which approximates the anted-diagonal structure of $C$ induced by the partiality. 
The term weighted by $\mu_2$ promotes orthogonality of the map by penalizing the off-diagonal entries of $C^{\top}C$.
Finally $d_{\ell} \in \{0, 1\}, \ \forall \ell$, and the ones equal to $1$ represent the singular values of $C$ that are expected to be non-zero. 

\textbf{Comparisons with GRASP?}

\subsection{Failure cases}
As we demonstrate empirically, this behavior is not universal across all types of graphs

\subsection{Regularizing effect} Nel main abbiamo scritto qualche volta che la C ha un regularizing effect, con il quale intendiamo che se la mappa o il segnale sono rumorosi, abbiamo low pass aggratis. Inoltre e' ben definita anche nel caso non punto-punto. Dobbiamo supportare questi claim con qualche test.
