# Supplementary material for: Spectral Maps for Learning on Subgraphs
Source: arXiv:2205.14938 source file (2023-01-31)
Supplement: Supplementary file 2 [file ablation_C.tex]

\section{\label{sec:add_exp}Additional experiments}

\begin{figure}[t]
\begin{subfigure}[b]{0.48\linewidth}
\centering
\begin{overpic}
[trim=0cm 0cm 0cm 0cm, clip,width=0.999\linewidth, grid=false]{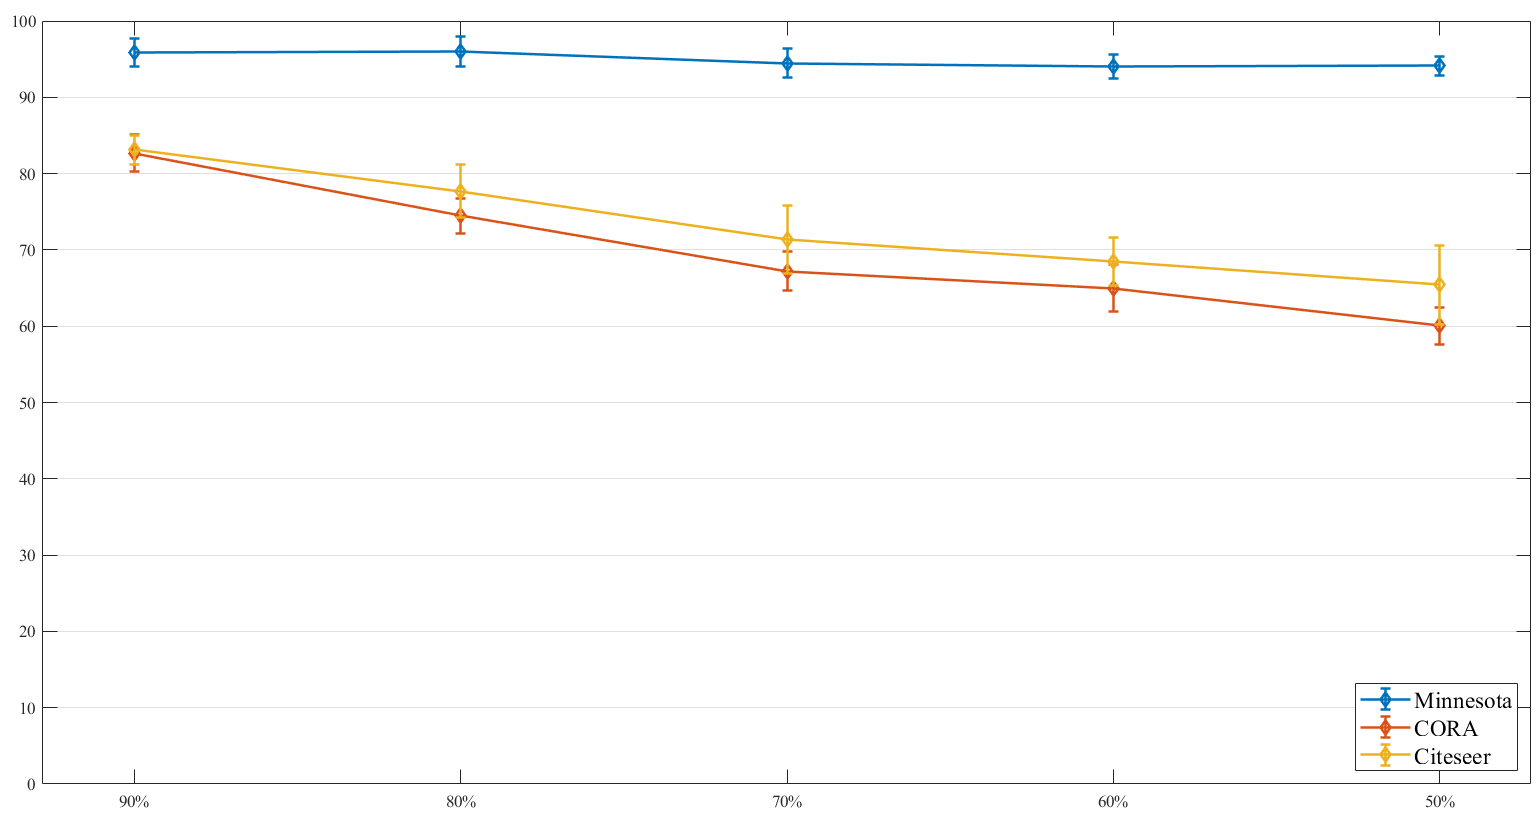}
\put(42,-2){\scriptsize Subgraph size}
\put(-3,36){\rotatebox[origin=c]{90}{\scriptsize MAP(\%)}}
\end{overpic}
\caption{\label{fig:n2n_subs_patch} Patch}
\end{subfigure}
\hfill
\begin{subfigure}[b]{0.48\linewidth}
\centering
\begin{overpic}
[trim=0cm 0cm 0cm 0cm,clip,width=0.999\linewidth, grid=false]{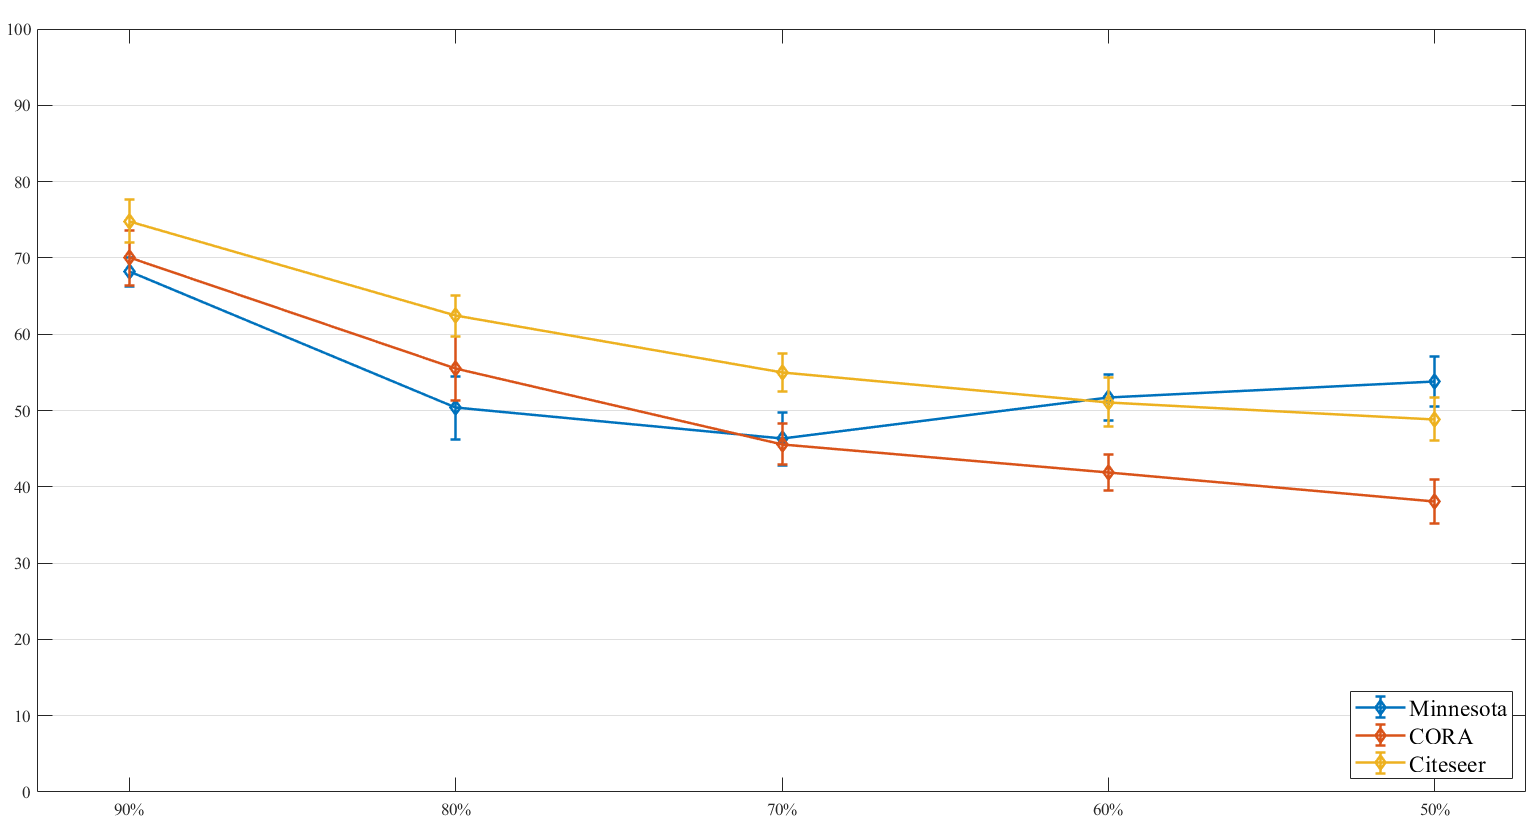}
\put(42,-2){\scriptsize Subgraph size}
\put(-3,36){\rotatebox[origin=c]{90}{\scriptsize MAP(\%)}}
\end{overpic}
\caption{\label{fig:n2n_subs_holes} Holes}
\end{subfigure}
\caption{\label{fig:n2n_subs} MAP(\%) of the correspondence on different datasets at decreasing size of the subgraph (expressed as percentages, decreasing from $90\%$ to $50\%$) with two types of partiality: patch (left) and holes (right). The correspondences are obtained from ground-truth spectral maps.}
\end{figure}

\subsection{Partiality percentage}
%How much the performance of the functional representation degrade with the dimension of the sub graph?
The aim of this experiment is to study how much the performance of the functional representation for a correspondence task degrades with different levels and types of partiality.

In Figure \ref{fig:n2n_subs}, we perform an experiment similar to the one in Section $5.3$ of the main paper and test how the MAP of the correspondence changes when we consider subgraphs of different dimensions. In particular, we test 2 partialities: patch and holes. The former is obtained by expanding a neighborhood from a given random node until a certain number of nodes is reached. The latter is obtained by removing random nodes with their immediate neighborhood.
The main difference is in the sparsity of the two partialities. The first keeps a cluster of nodes without changing the inner connectivity of the graph; the latter is sparser in the sense that it removes paths between nodes of the graph, changing the whole connectivity of the graph.
%{Devo ancora aggiungere l'immagine con le C dei vari casi così posso usare la struttura meno definita della C per giustificare il deterioramento delle performance}
{In Figure \ref{fig:partial}, we plot the spectral maps at different percentages of partiality of type patch (left) and holes (right).}
\begin{figure}[t]
\vspace{0.2cm}
\centering
\begin{subfigure}[b]{0.48\textwidth}
\centering
\begin{overpic}
[trim=0cm 0cm 0cm 0cm,clip,width=0.999\linewidth,grid=false]{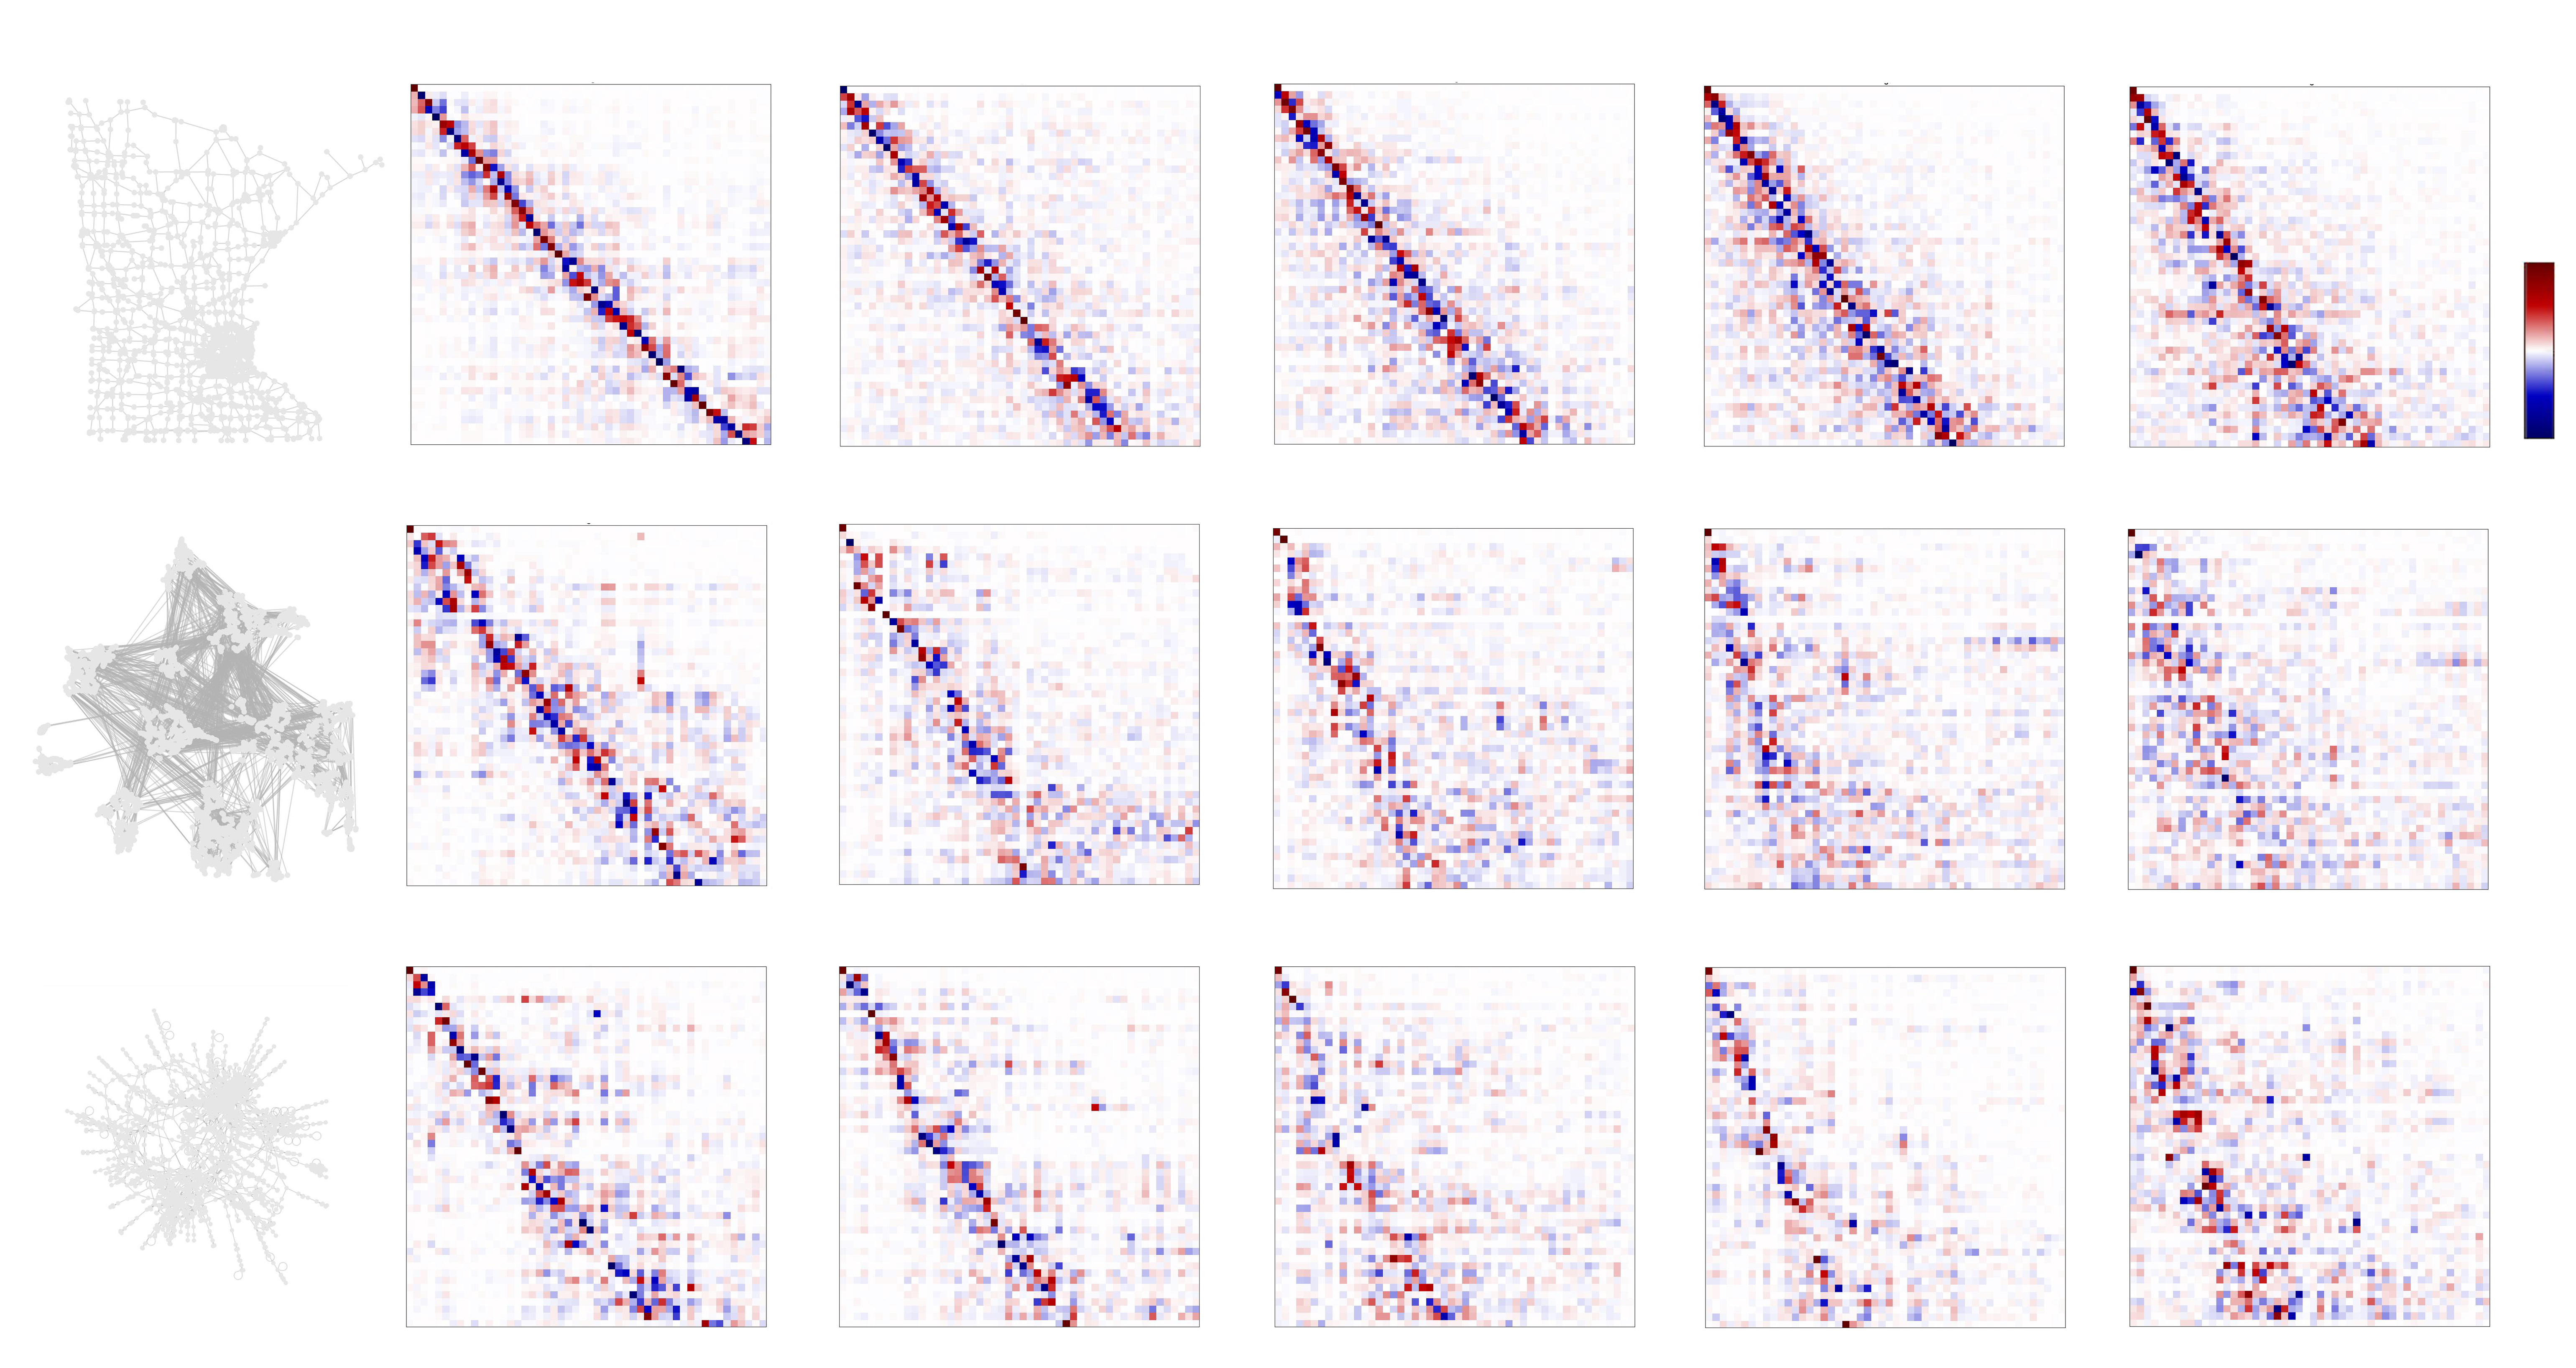}
\put(1,51){\tiny Minnesota}
\put(4,33){\tiny CORA}
\put(3,15){\tiny Citeseer}
\put(20,51){\tiny $90\%$}
\put(37,51){\tiny $80\%$}
\put(53,51){\tiny $70\%$}
\put(70,51){\tiny $60\%$}
\put(87,51){\tiny $50\%$}
\end{overpic}
\caption{\label{fig:patch} Patch}

\end{subfigure}
 \hfill
 \begin{subfigure}[b]{0.48\textwidth}
\centering
\begin{overpic}
[trim=0cm 0cm 0cm 0cm,clip,width=0.999\linewidth]{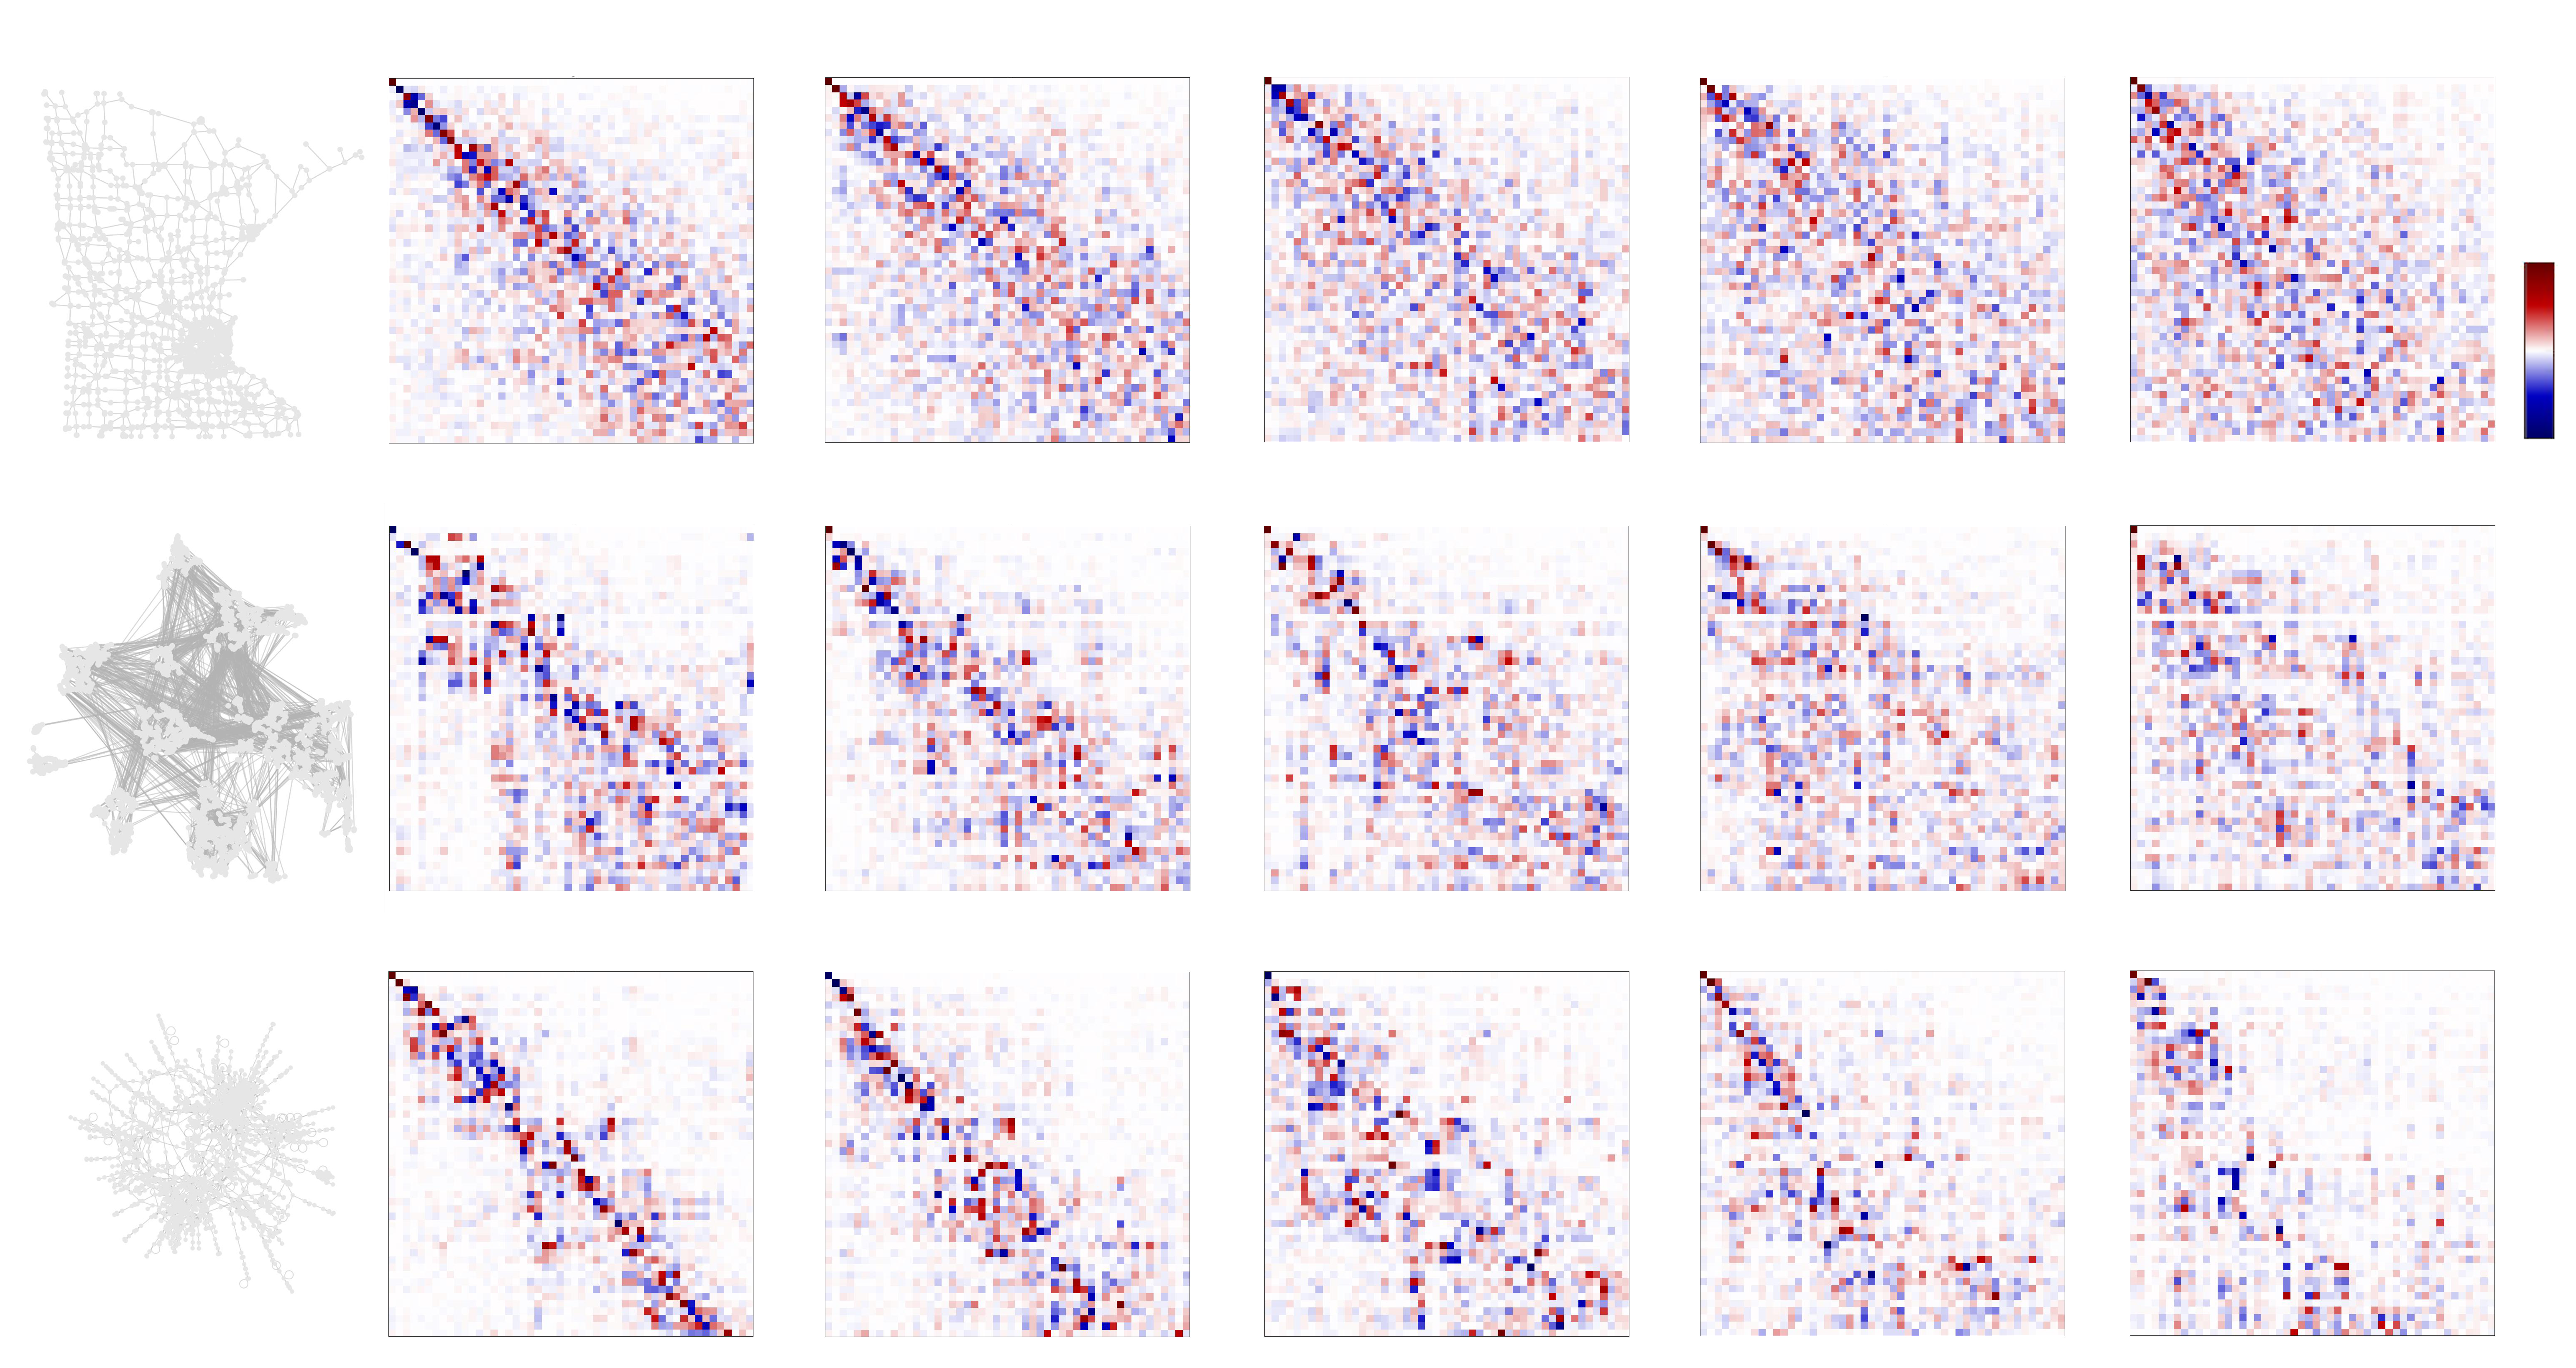}
\put(1,51){\tiny Minnesota}
\put(4,33){\tiny CORA}
\put(3,15){\tiny Citeseer}
\put(20,51){\tiny $90\%$}
\put(37,51){\tiny $80\%$}
\put(53,51){\tiny $70\%$}
\put(70,51){\tiny $60\%$}
\put(87,51){\tiny $50\%$}
\end{overpic}
\caption{\label{fig:holes} Holes}
\end{subfigure}
 \hfill
\caption{\label{fig:partial} Robustness of the map to the action of two partialities: patch and holes. The partialities are increasingly wider, from a subgraph with $90\%$ of the nodes to a subgraph with $50\%$ of the nodes. As partiality increases, the functional map structure becomes less defined.}
\end{figure}

%\subsection{Partiality diffusion}
%Consider a different kind of partiality: holes. Compared to the cut/patch where the remaining sub graph has its connectivity almost intact, it's a more widespread partiality. 

% \subsection{\label{sec:nume_eig}Number of eigenvectors}
% In Figure~\ref{fig:n2n_eigs}, we report the correspondence accuracy obtained from ground-truth spectral maps ($GT$ in the main paper) under increasing percentage of eigenvectors.

\subsection{\label{sec:add_rewire}Rewiring}
In the main paper and in Figure~\ref{fig:graphsRewiring}, we highlight how the spectral map degrades when we apply a sequence of local rewiring operations. Here we consider a much stronger variation, namely, a {\em global} rewiring where we do not limit the topological perturbation to a local neighborhood. The results are reported in Figure~\ref{fig:graphsRewiringHops}.

\begin{figure}[t]
\vspace{0.2cm}
\centering
\begin{overpic}
[trim=0cm 0cm 0cm 0cm,clip,width=0.999\linewidth,grid=False]{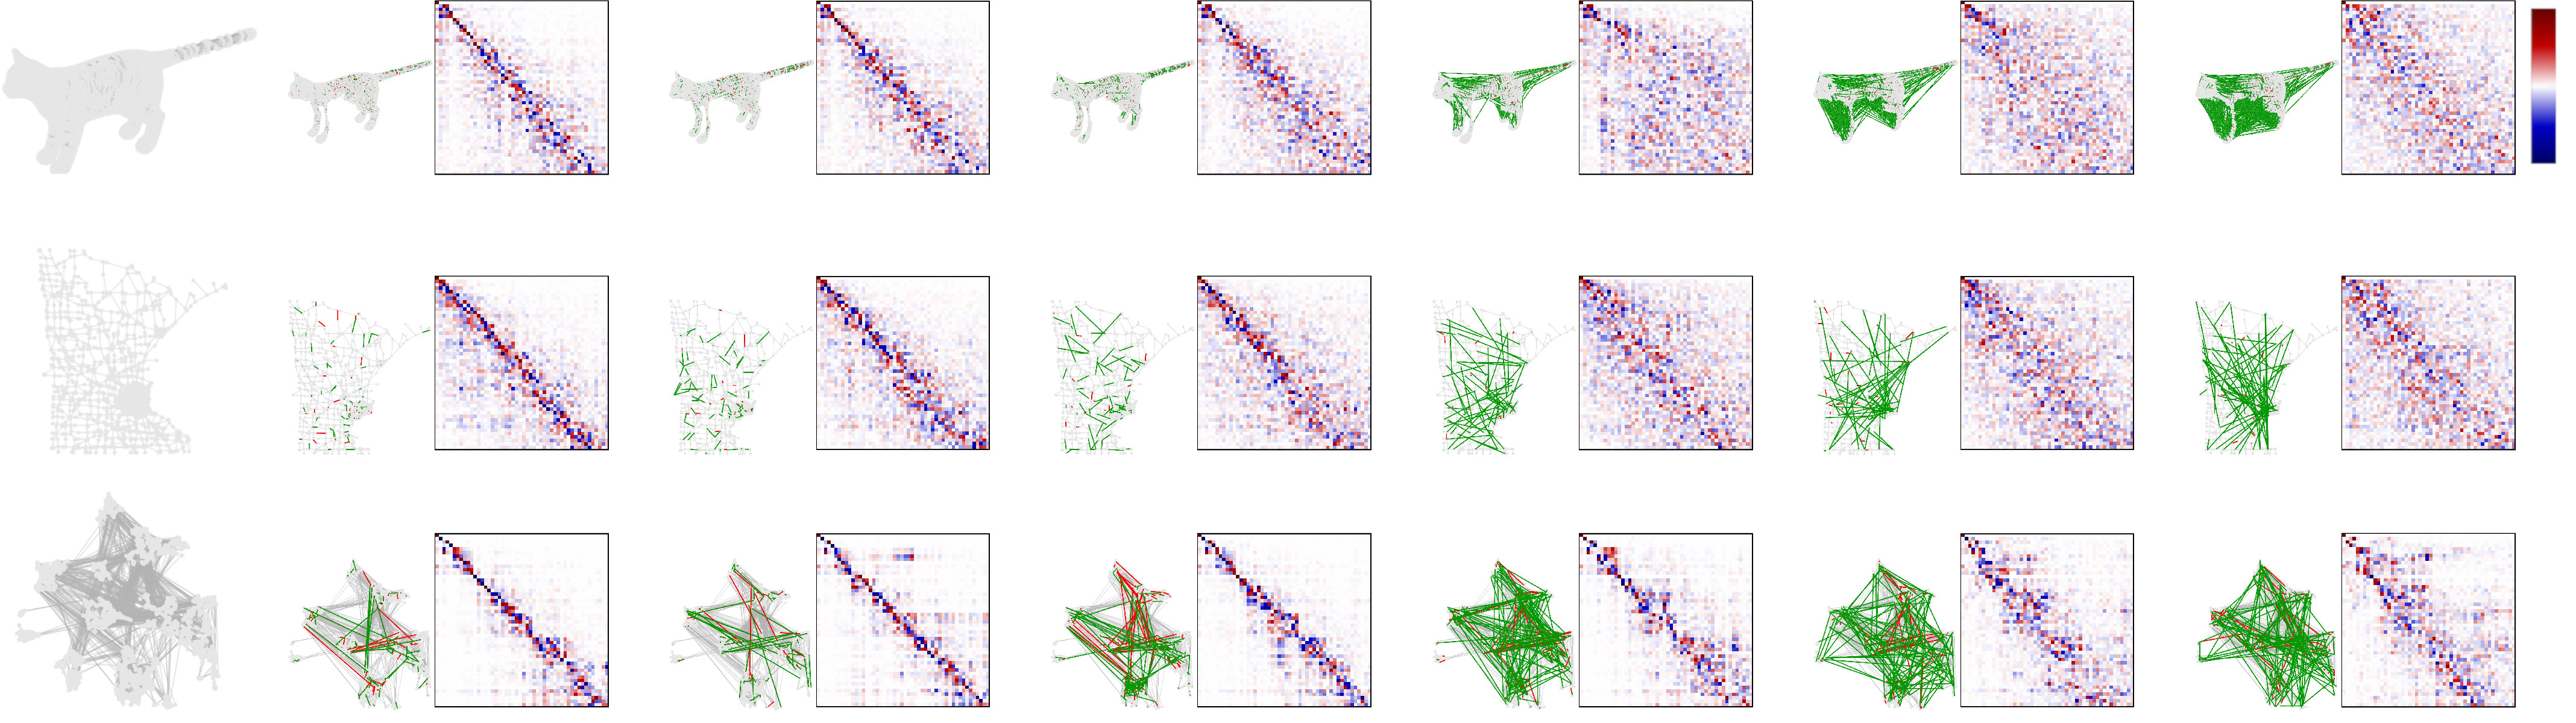}
\put(-2,28.0){\tiny Cat}
\put(-2,18.7){\tiny Minnesota}
\put(-2,8.0){\tiny CORA}
\put(99.7,27.0){\tiny $1$}
\put(99.6,21.9){\tiny $\scalebox{0.7}[1.0]{-}1$}
\put(16.0,28.5){\tiny $1\%$}
\put(31,28.5){\tiny $5\%$}
\put(45.5,28.5){\tiny $10\%$}
\put(60.2,28.5){\tiny $30\%$}
\put(74.8,28.5){\tiny $50\%$}
\put(89.3,28.5){\tiny $100\%$}
\put(16.0,18.2){\tiny $1\%$}
\put(31,18.2){\tiny $5\%$}
\put(45.5,18.2){\tiny $10\%$}
\put(60.2,18.2){\tiny $30\%$}
\put(74.8,18.2){\tiny $50\%$}
\put(89.3,18.2){\tiny $100\%$}
\put(16.0,8.0){\tiny $1\%$}
\put(31,8.0){\tiny $5\%$}
\put(45.5,8.0){\tiny $10\%$}
\put(60.2,8.0){\tiny $30\%$}
\put(74.8,8.0){\tiny $50\%$}
\put(89.3,8.0){\tiny $100\%$}
\end{overpic}
\caption{\label{fig:graphsRewiringHops} Robustness of the map to the simultaneous action of partiality and rewiring of the subgraph. The rewiring operations are increasingly \textbf{wider}, involving nodes and edges farther apart. The left column shows the full graph, while the pairs composed by a graph and a matrix show the rewiring operation and the resulting spectral map, starting with a rewiring involving just nodes within $1\%$ of the graph diameter (left) up to the full graph diameter (right).}
\end{figure}
\begin{figure}[t]
\vspace{0.2cm}
\centering
\begin{overpic}
[trim=0cm 0cm 0cm 0cm,clip,width=0.999\linewidth, grid=false]{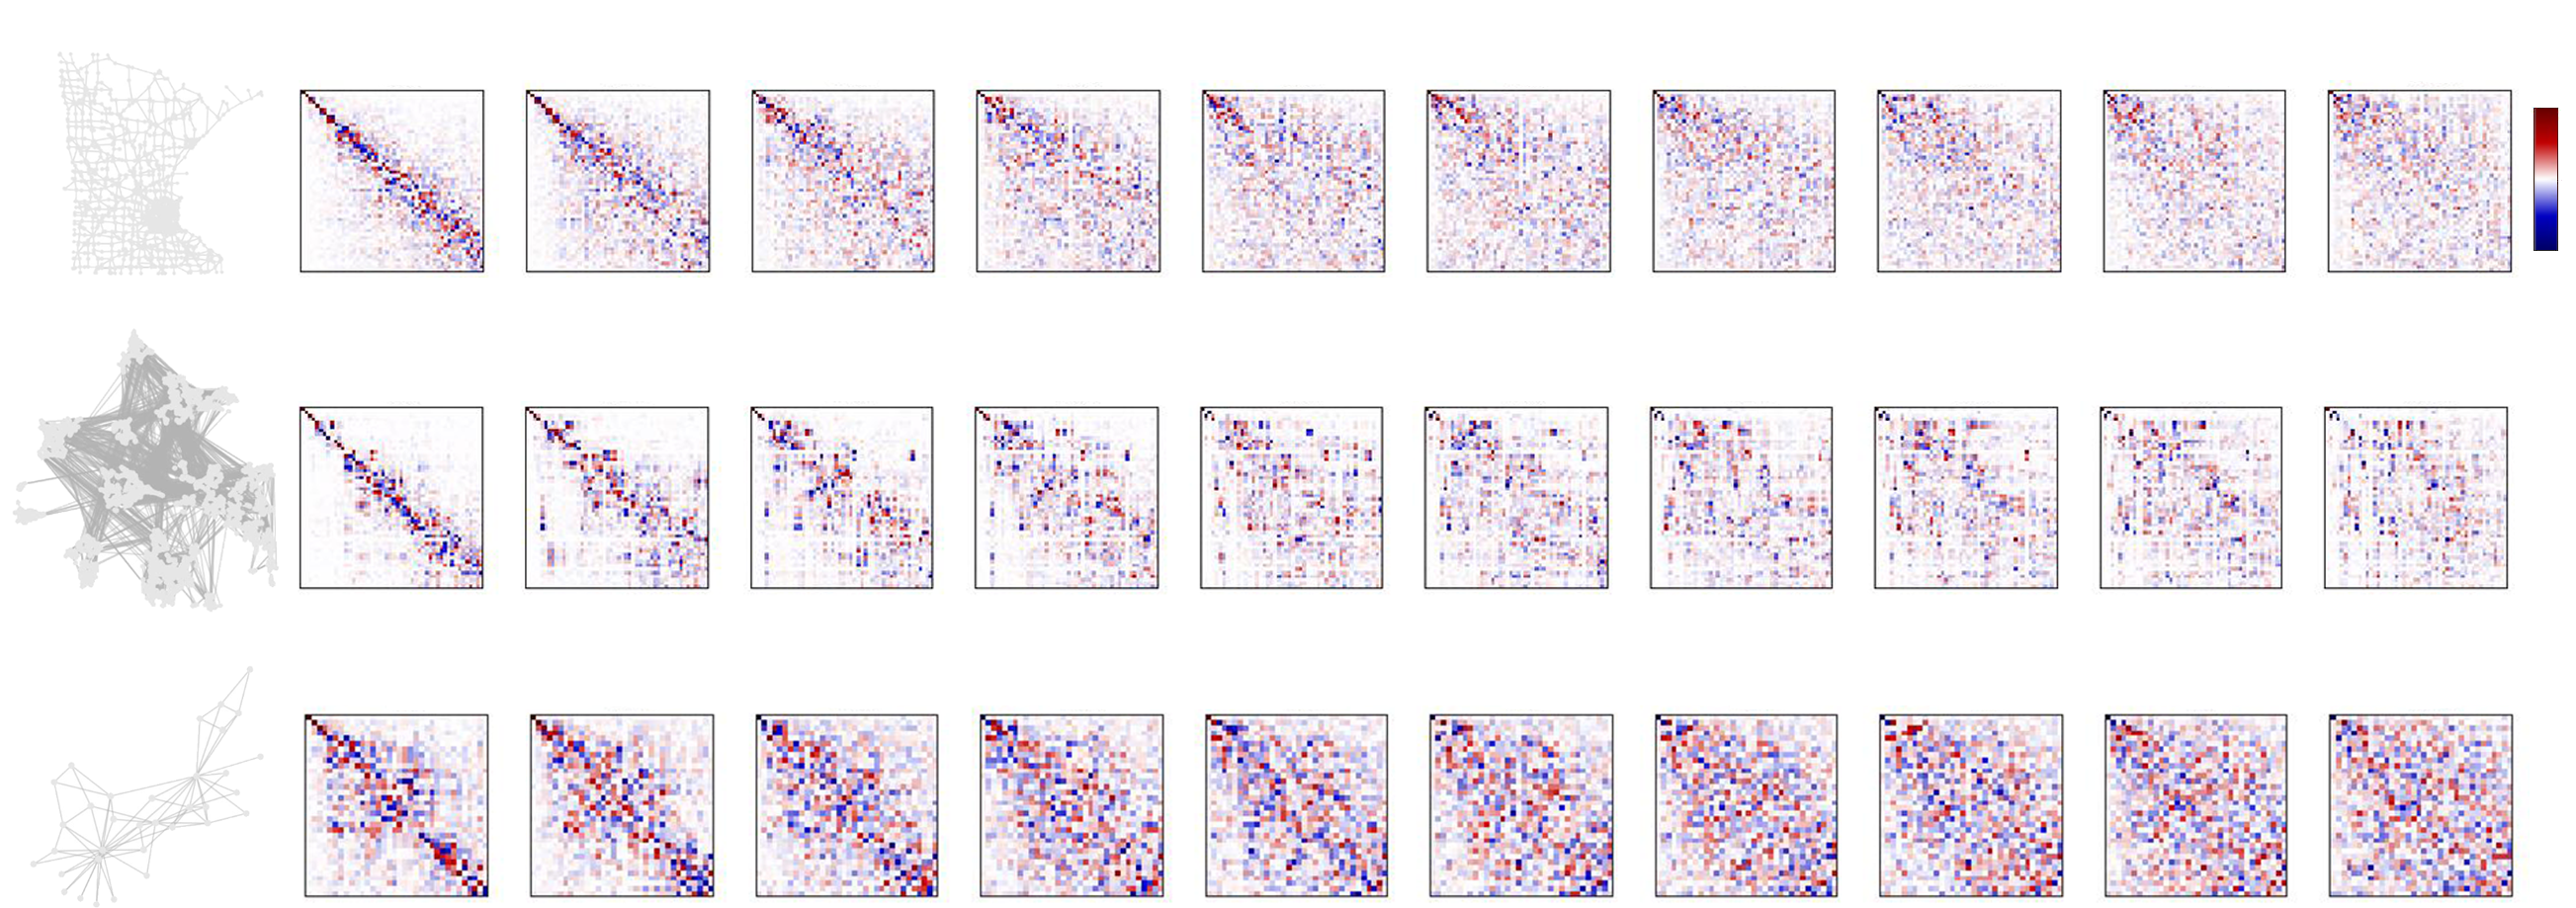}
\put(2,34){\tiny Minnesota}
\put(4,23){\tiny CORA}
\put(4,9){\tiny Karate}
\put(100,31){\tiny $1$}
\put(100,25){\tiny $\scalebox{0.7}[1.0]{-}1$}
\put(14.5,32){\tiny $8\%$}
\put(22.5,32){\tiny $16\%$}
\put(31.5,32){\tiny $24\%$}
\put(40,32){\tiny $32\%$}
\put(49,32){\tiny $40\%$}
\put(57.5,32){\tiny $48\%$}
\put(66.5,32){\tiny $56\%$}
\put(75.5,32){\tiny $64\%$}
\put(84,32){\tiny $72\%$}
\put(92.5,32){\tiny $80\%$}
\put(14.5,19.7){\tiny $8\%$}
\put(22.5,19.7){\tiny $16\%$}
\put(31.5,19.7){\tiny $24\%$}
\put(40,19.7){\tiny $32\%$}
\put(49,19.7){\tiny $40\%$}
\put(57.5,19.7){\tiny $48\%$}
\put(66.5,19.7){\tiny $56\%$}
\put(75.5,19.7){\tiny $64\%$}
\put(84,19.7){\tiny $72\%$}
\put(92.5,19.7){\tiny $80\%$}
\put(14.5,7.7){\tiny $8\%$}
\put(22.5,7.7){\tiny $16\%$}
\put(31.5,7.7){\tiny $24\%$}
\put(40,7.7){\tiny $32\%$}
\put(49,7.7){\tiny $40\%$}
\put(57.5,7.7){\tiny $48\%$}
\put(66.5,7.7){\tiny $56\%$}
\put(75.5,7.7){\tiny $64\%$}
\put(84,7.7){\tiny $72\%$}
\put(92.5,7.7){\tiny $80\%$}
\end{overpic}
\caption{\label{fig:graphsOnlyRewiringInc} Robustness of the map to rewiring of the subgraph.
The rewiring operations are increasingly stronger, with increments of 8\% of the total number of
edges (starting from 8\% and reaching 80\%). The plotted matrices represent the functional map after the topological perturbations, showing the effect
of rewiring on the functional map structure.}
\end{figure}
\begin{figure}[t]
\vspace{0.2cm}
\centering
\begin{overpic}
[trim=0cm 0cm 0cm 0cm,clip,width=0.999\linewidth, grid=false]{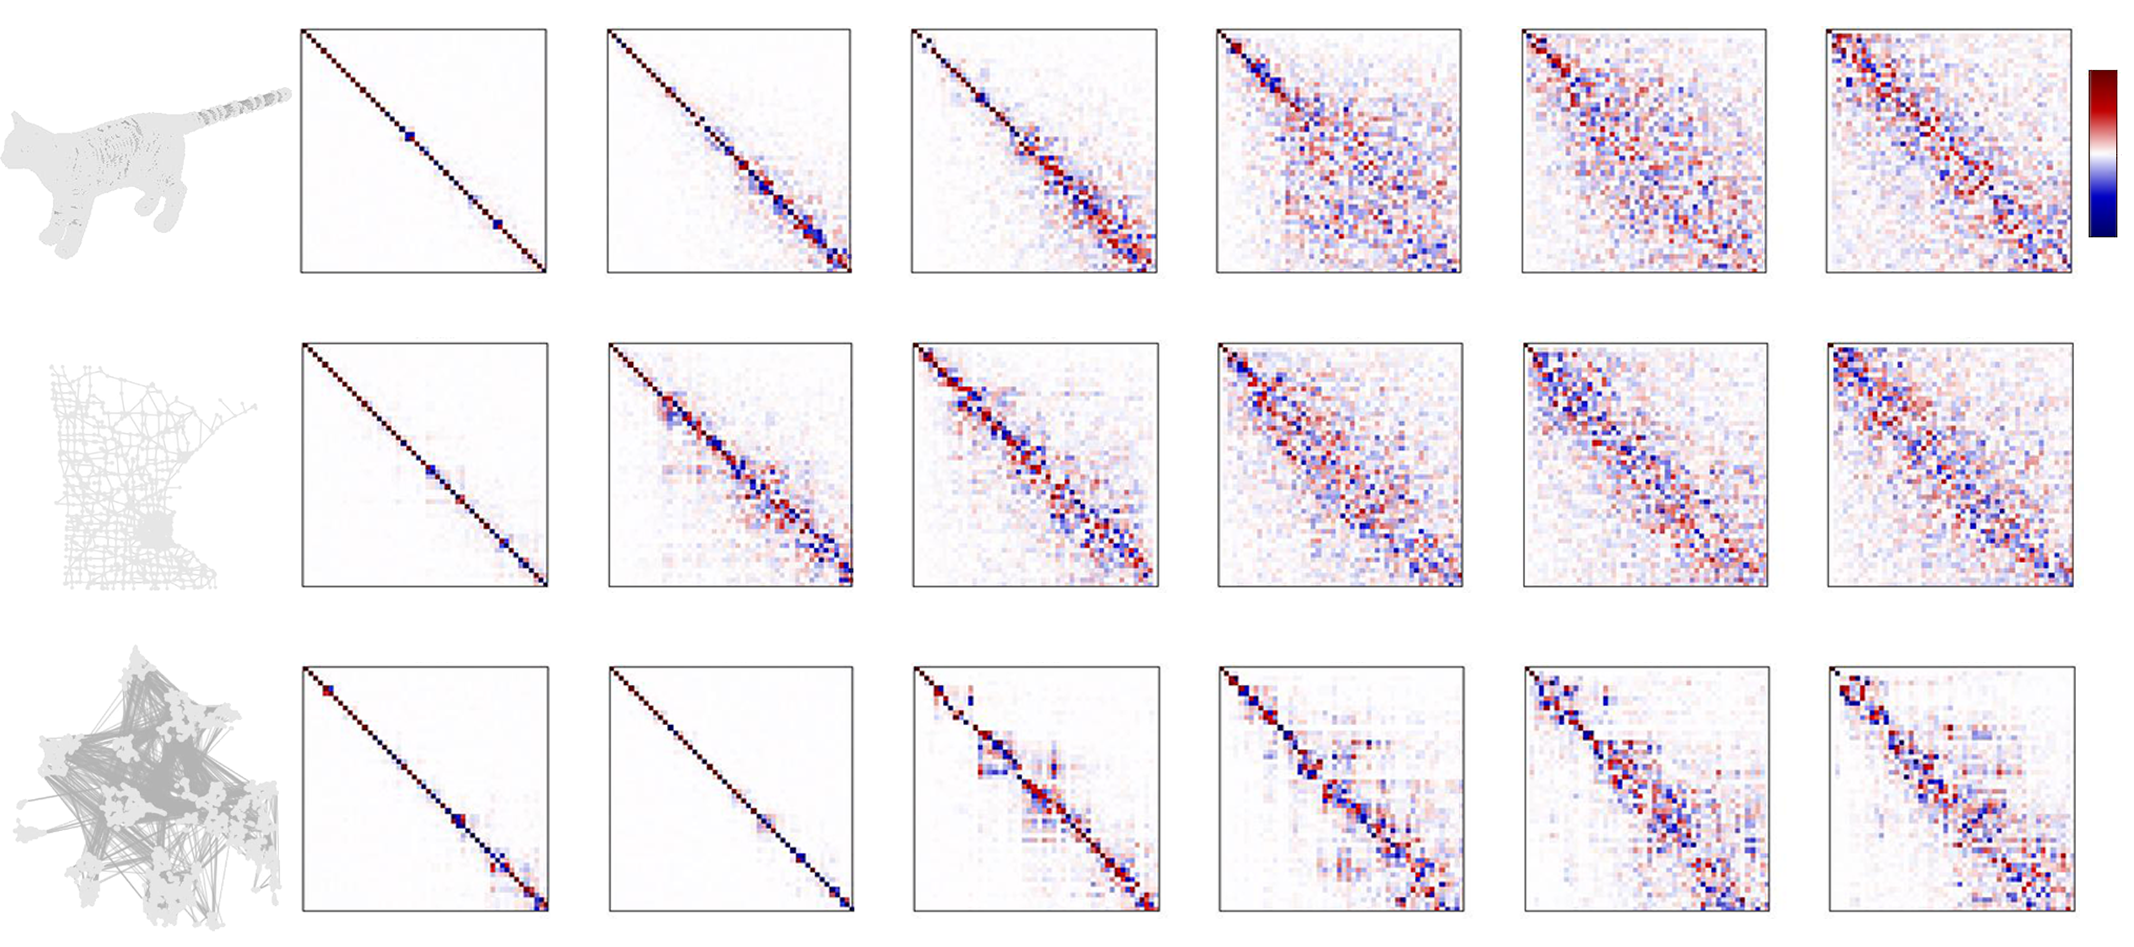}
\put(5,40){\tiny cat}
\put(3,28.5){\tiny Minnesota}
\put(5,15){\tiny CORA}
\put(100,41){\tiny $1$}
\put(100,32.5){\tiny $\scalebox{0.7}[1.0]{-}1$}
\put(19,43.5){\tiny $1\%$}
\put(33,43.5){\tiny $5\%$}
\put(47.5,43.5){\tiny $10\%$}
\put(61.5,43.5){\tiny $30\%$}
\put(76,43.5){\tiny $50\%$}
\put(90,43.5){\tiny $100\%$}
\put(19,28.5){\tiny $1\%$}
\put(33,28.5){\tiny $5\%$}
\put(47.5,28.5){\tiny $10\%$}
\put(61.5,28.5){\tiny $30\%$}
\put(76,28.5){\tiny $50\%$}
\put(90,28.5){\tiny $100\%$}
\put(19,13.5){\tiny $1\%$}
\put(33,13.5){\tiny $5\%$}
\put(47.5,13.5){\tiny $10\%$}
\put(61.5,13.5){\tiny $30\%$}
\put(76,13.5){\tiny $50\%$}
\put(90,13.5){\tiny $100\%$}
\end{overpic}
\caption{\label{fig:graphsOnlyRewiringWider} Robustness of the map to rewiring of the subgraph.
The rewiring operations are increasingly wider, involving nodes and edges farther apart. The left
column shows the full graph, while the others columns show the resulting functional map, starting with a rewiring involving just nodes within 1\% of
the graph diameter (left) up to the full graph diameter (right)}
\end{figure}
{Finally, in Figures \ref{fig:graphsOnlyRewiringInc} and \ref{fig:graphsOnlyRewiringWider}, we show the spectral maps under the action of pure rewiring perturbations, without any partiality involved.}

%\subsection{Number of eigenvectors}\label{sec:nevals}
%
%In all the experiments we had used only the first 50 eigenvectors of the normalized graph laplacian. 
%Here we test the performance improvement when more than 50 eigenvectors are used in order to understand the best trade off between number of eigenvectors and performance

% \begin{figure}[h!]
% % \vspace{0.0cm}
% \centering
% \begin{overpic}
% [trim=0cm 0cm 0cm 0cm,clip,width=0.8\linewidth]{./figures/Amazon_Photo.jpg}
% \end{overpic}
% \caption{\label{fig:AmazonPhoto500} spectral map between AmazonPhoto and its partial graph: left has size $500\times500$, left $100\times100$.{Add other visual examples: Cora }}
% \end{figure}

%\input{sections/Tabels/TAB_k_increase}

% \subsection{spectral map from not well defined n2n correspondences}
% In the main manuscript, we have only considered cases where an exact node to node correspondences is defined, but this is not always the case (see PPI align). In this section we want to see and test how the functional repsesentation behave in those cases where the correspondence between nodes in a graph is not well defined (not an injection).
